# Supplementary material for: Diffusion-based Human Motion Style Transfer with Semantic Guidance
Source: arXiv:2405.06646 source file (2024-08-07)
Supplement: Supplementary file 1 [file zappendix.tex]

% ---------------------------------------------------------------------------
% Author guideline and sample document for EG publication using LaTeX2e input
% D.Fellner, v1.22, Jan 22, 2024

\documentclass{egpubl}
\usepackage{sca2024}
\usepackage{amssymb}
\usepackage{amsmath}
\usepackage{multirow}

% \usepackage[numbers]{natbib}

% \usepackage{natbib} 
% --- for  Annual CONFERENCE
% \ConferenceSubmission   % uncomment for Conference submission
% \ConferencePaper        % uncomment for (final) Conference Paper
% \STAR                   % uncomment for STAR contribution
% \Tutorial               % uncomment for Tutorial contribution
% \ShortPresentation      % uncomment for (final) Short Conference Presentation
% \Areas                  % uncomment for Areas contribution
% \Education              % uncomment for Education contribution
% \Poster                 % uncomment for Poster contribution
% \DC                     % uncomment for Doctoral Consortium
%
% --- for  CGF Journal
% \JournalSubmission    % uncomment for submission to Computer Graphics Forum
% \JournalPaper         % uncomment for final version of Journal Paper
%
% --- for  CGF Journal: special issue
% \SpecialIssueSubmission    % uncomment for submission to , special issue
\SpecialIssuePaper         % uncomment for final version of Computer Graphics Forum, special issue
%                          % EuroVis, SGP, Rendering, PG
% --- for  EG Workshop Proceedings
% \WsSubmission      % uncomment for submission to EG Workshop
% \WsPaper           % uncomment for final version of EG Workshop contribution
% \WsSubmissionJoint % for joint events, for example ICAT-EGVE
% \WsPaperJoint      % for joint events, for example ICAT-EGVE
% \WsPaperJointdemo         % uncomment for final version of EG Workshop contribution
% \WsPaperJointposter         % uncomment for final version of EG Workshop contribution 
% \WsPoster          % uncomment for Poster contribution
% \SpecialIssuePaper
% \WsShortPaper      % uncomment for Short Paper contribution
% \Expressive        % for SBIM, CAe, NPAR
% \DigitalHeritagePaper
% \PaperL2P          % for events EG only asks for License to Publish

% --- for EuroVis 
% for full papers use \SpecialIssuePaper
% \STAREurovis   % for EuroVis additional material 
% \EuroVisPoster % for EuroVis additional material 
% \EuroVisShort  % for EuroVis additional material
% \MedicalPrize  % uncomment for Medical Prize (Dirk Bartz) contribution, since 2021 part of EuroVis
% \EuroVisEducation              % uncomment for Education contribution

% Licences: for CGF Journal (EG conf. full papers and STARs, EuroVis conf. full papers and STARs, SR, SGP, PG)
% please choose the correct license
%\CGFStandardLicense
\CGFccby
%\CGFccbync
%\CGFccbyncnd

% !! *please* don't change anything above
% !! unless you REALLY know what you are doing
% ------------------------------------------------------------------------
\usepackage[T1]{fontenc}
\usepackage{dfadobe}  

\usepackage{cite}  % comment out for biblatex with backend=biber

\usepackage{xcolor}

% ---------------------------
%\biberVersion
\BibtexOrBiblatex
%\usepackage[backend=biber,bibstyle=EG,citestyle=alphabetic,backref=true]{biblatex} 
%\addbibresource{egbibsample.bib}
% ---------------------------  
\electronicVersion
\PrintedOrElectronic
% for including postscript figures
% mind: package option 'draft' will replace PS figure by a filename within a frame
\ifpdf \usepackage[pdftex]{graphicx} \pdfcompresslevel=9
\else \usepackage[dvips]{graphicx} \fi

\usepackage{egweblnk} 
% end of prologue

\usepackage{graphicx}
\usepackage{multirow}
\usepackage{multicol}
\usepackage{makecell}
\usepackage{cuted}
\usepackage{indentfirst}

\input{zappendix.inc}
