# Supplementary material for: Diffusion-based Human Motion Style Transfer with Semantic Guidance
Source: arXiv:2405.06646 source file (2024-08-07)
Supplement: Supplementary file 2 [file appendix_content.tex]

\section{Qualitative Style Transfer Results on Bandai-2 Test Set}
Figure~\ref{fig:qualitative_comparison_bandai} presents a comparative example of human motion style transfer on the Bandai-2 test set. The input content motion is \textit{"wave right hand neutral"}, while the style motion is \textit{"raise left hand masculine"}. Across all methods, the outcomes exhibit masculine stylistic attributes, characterized by a wide-legged stance with one hand akimbo. Our results accurately preserve the input content details, with the trajectory of the right-hand wave aligning seamlessly with the input content. In contrast, while UMST and MotionPuzzle yield a commendable masculine style, they encounter difficulties in preserving the motion content in this case. Specifically, the character in their results continues to wave the left hand despite the input content specifying a right-hand wave.
Although FineStyle correctly distinguishes between the left and right arms, it generates movements that raise the right hand instead of waving it. These results suggest that the AdaIN-based motion style transfer methods may lead to confusion between content and style motions due to the non-interpretability of content-style disentanglement. However, our approach treats style transfer as a motion translation problem in the diffusion model, thus achieving better content preservation. 

\begin{figure}[t]
    \centering
    \includegraphics[width=\linewidth]{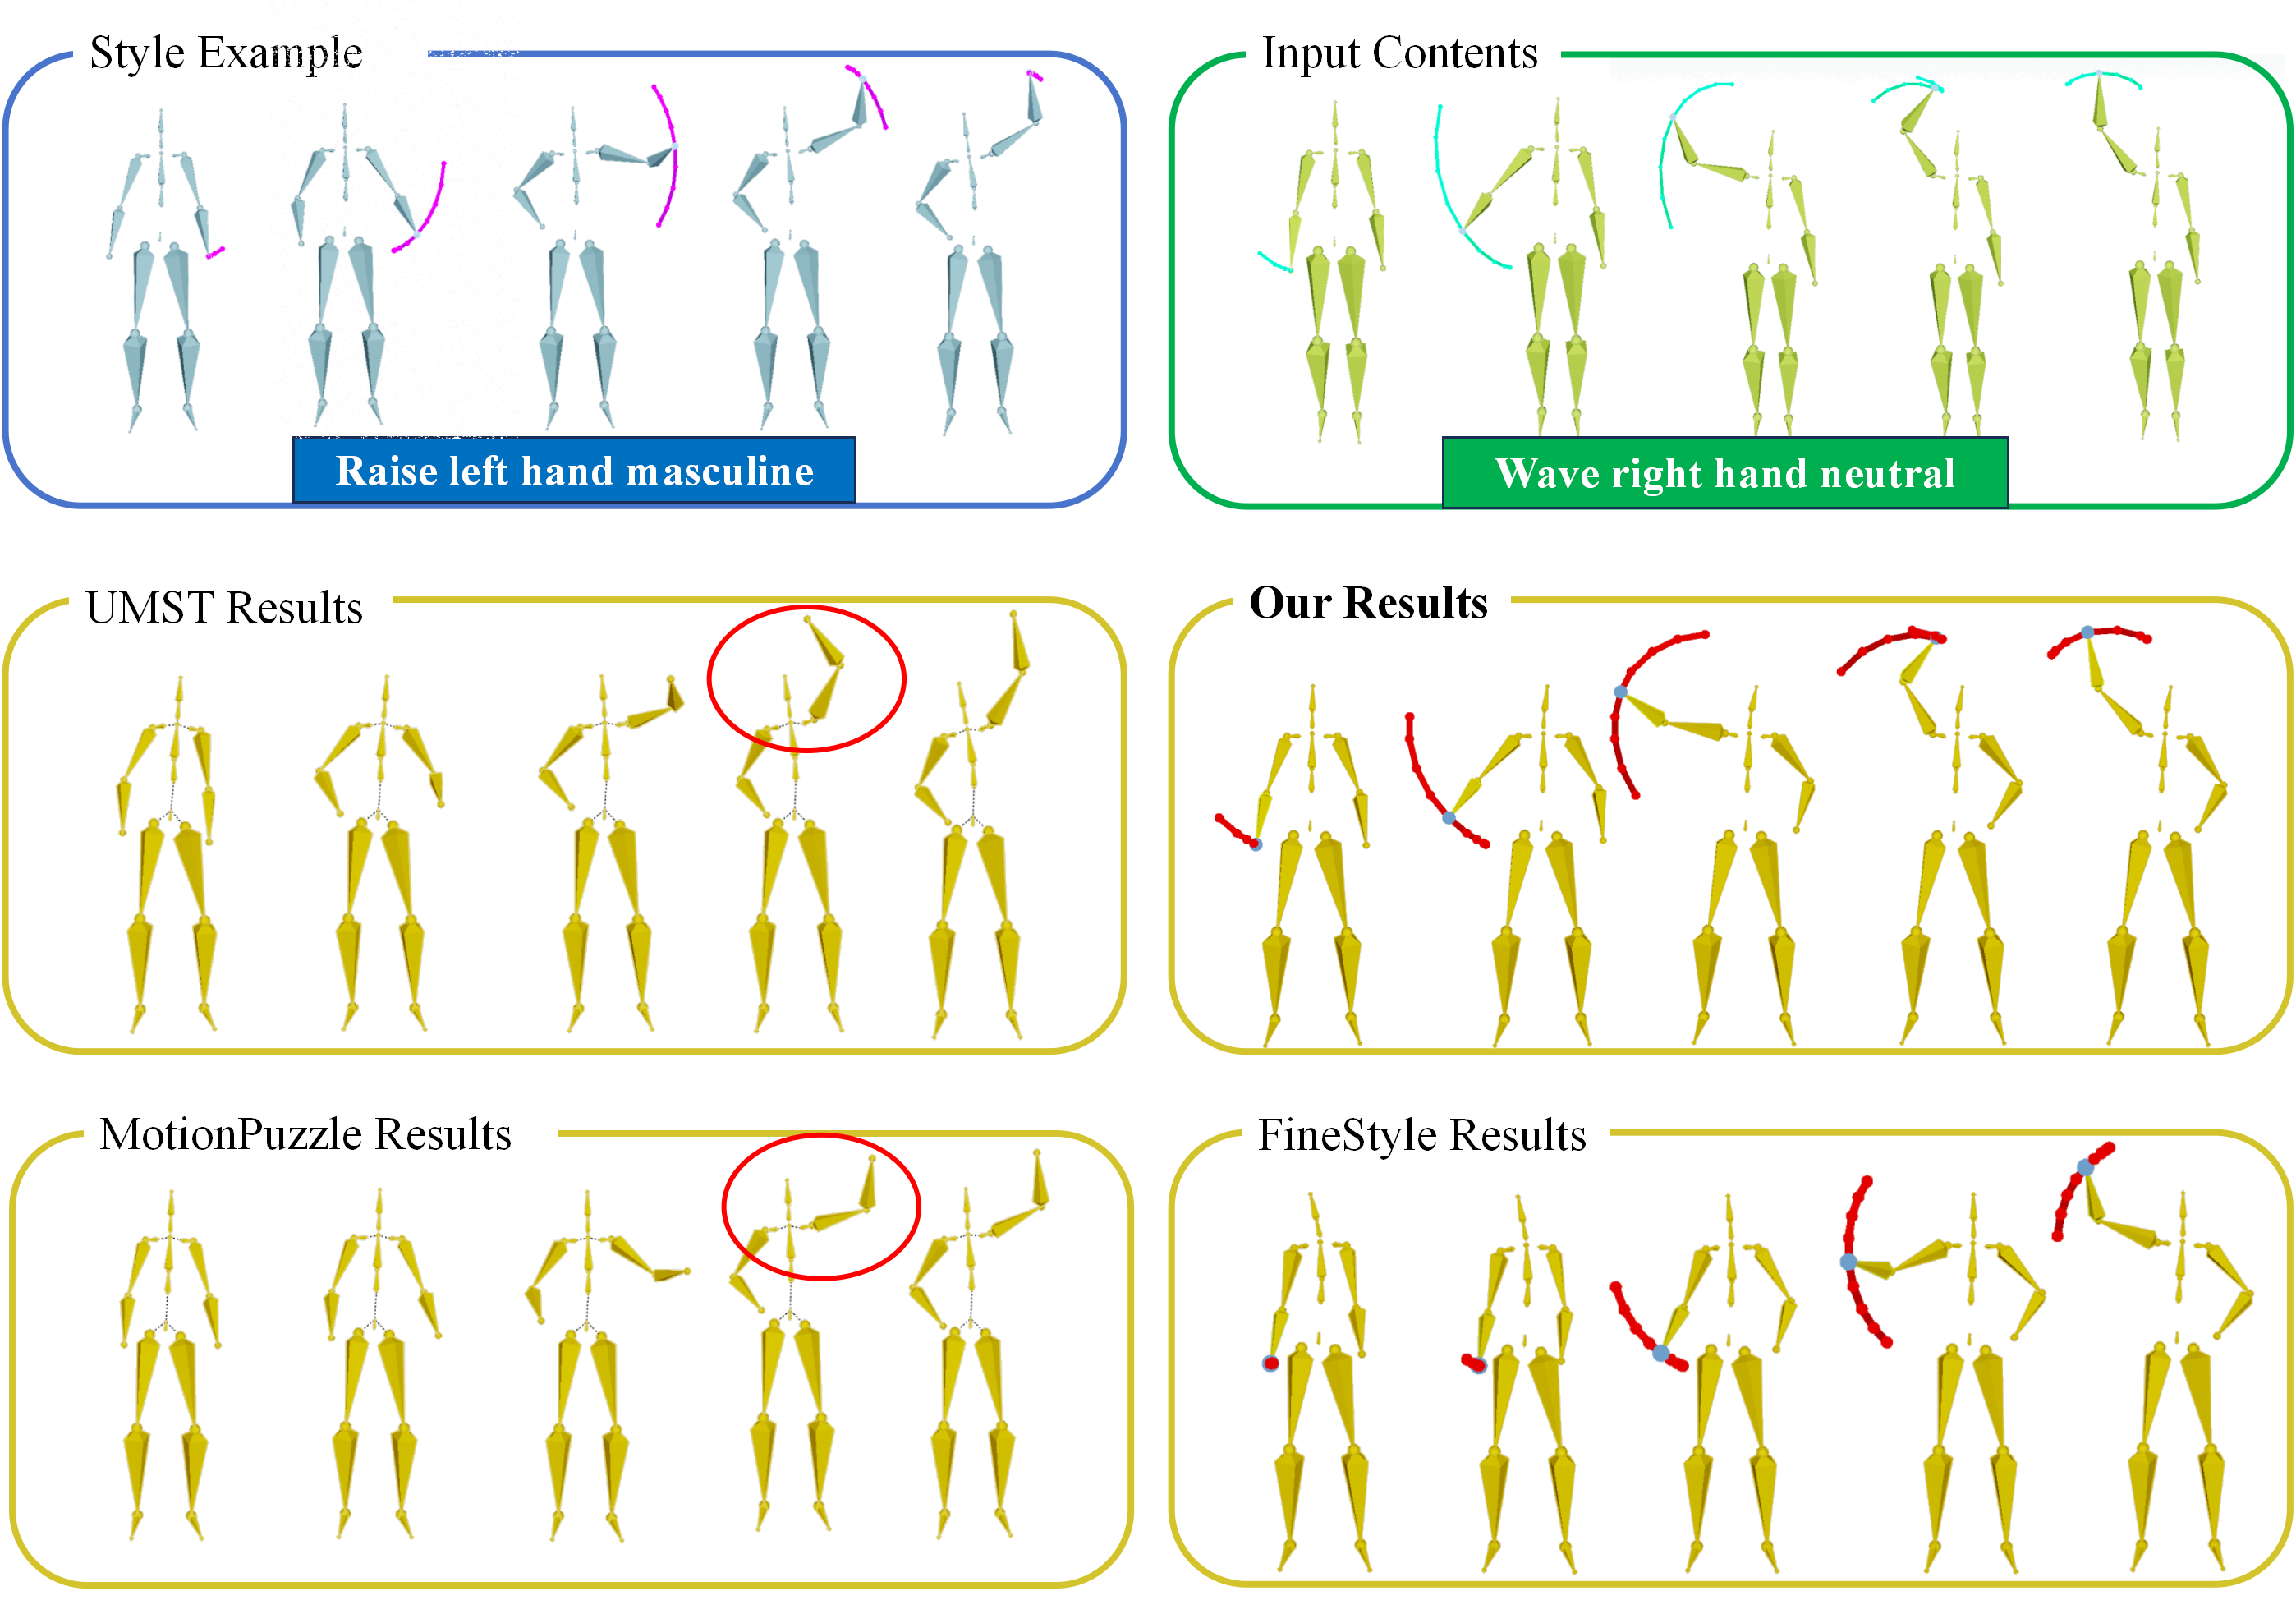}
    \caption{Qualitative results on the Bandai-2 test set. The curve in the figure represents the trajectory of the end-effector between -0.2s$\sim$0.2s. Flaws are marked by red circles.}
    \label{fig:qualitative_comparison_bandai}
\end{figure}

\section{Qualitative Results on Paired Neutral Motion Generation}

Our system uses the generative prior $\varepsilon_\theta$ to generate the paired neutral motion $m^{s\_n}$ corresponding to the input style example $m^s$. We compare the qualitative results with KNN+DTW. From Figure~\ref{fig:style_neutral_pairs}, our method can achieve a promising neutral motion generation performance. In comparison with KNN+DTW, the neutral motion poses produced by our generative prior $\varepsilon_\theta$ are similar to the motions in the dataset and can be well aligned with the input style example in terms of timing.

\begin{figure}
    \centering
    \includegraphics[width=\linewidth]{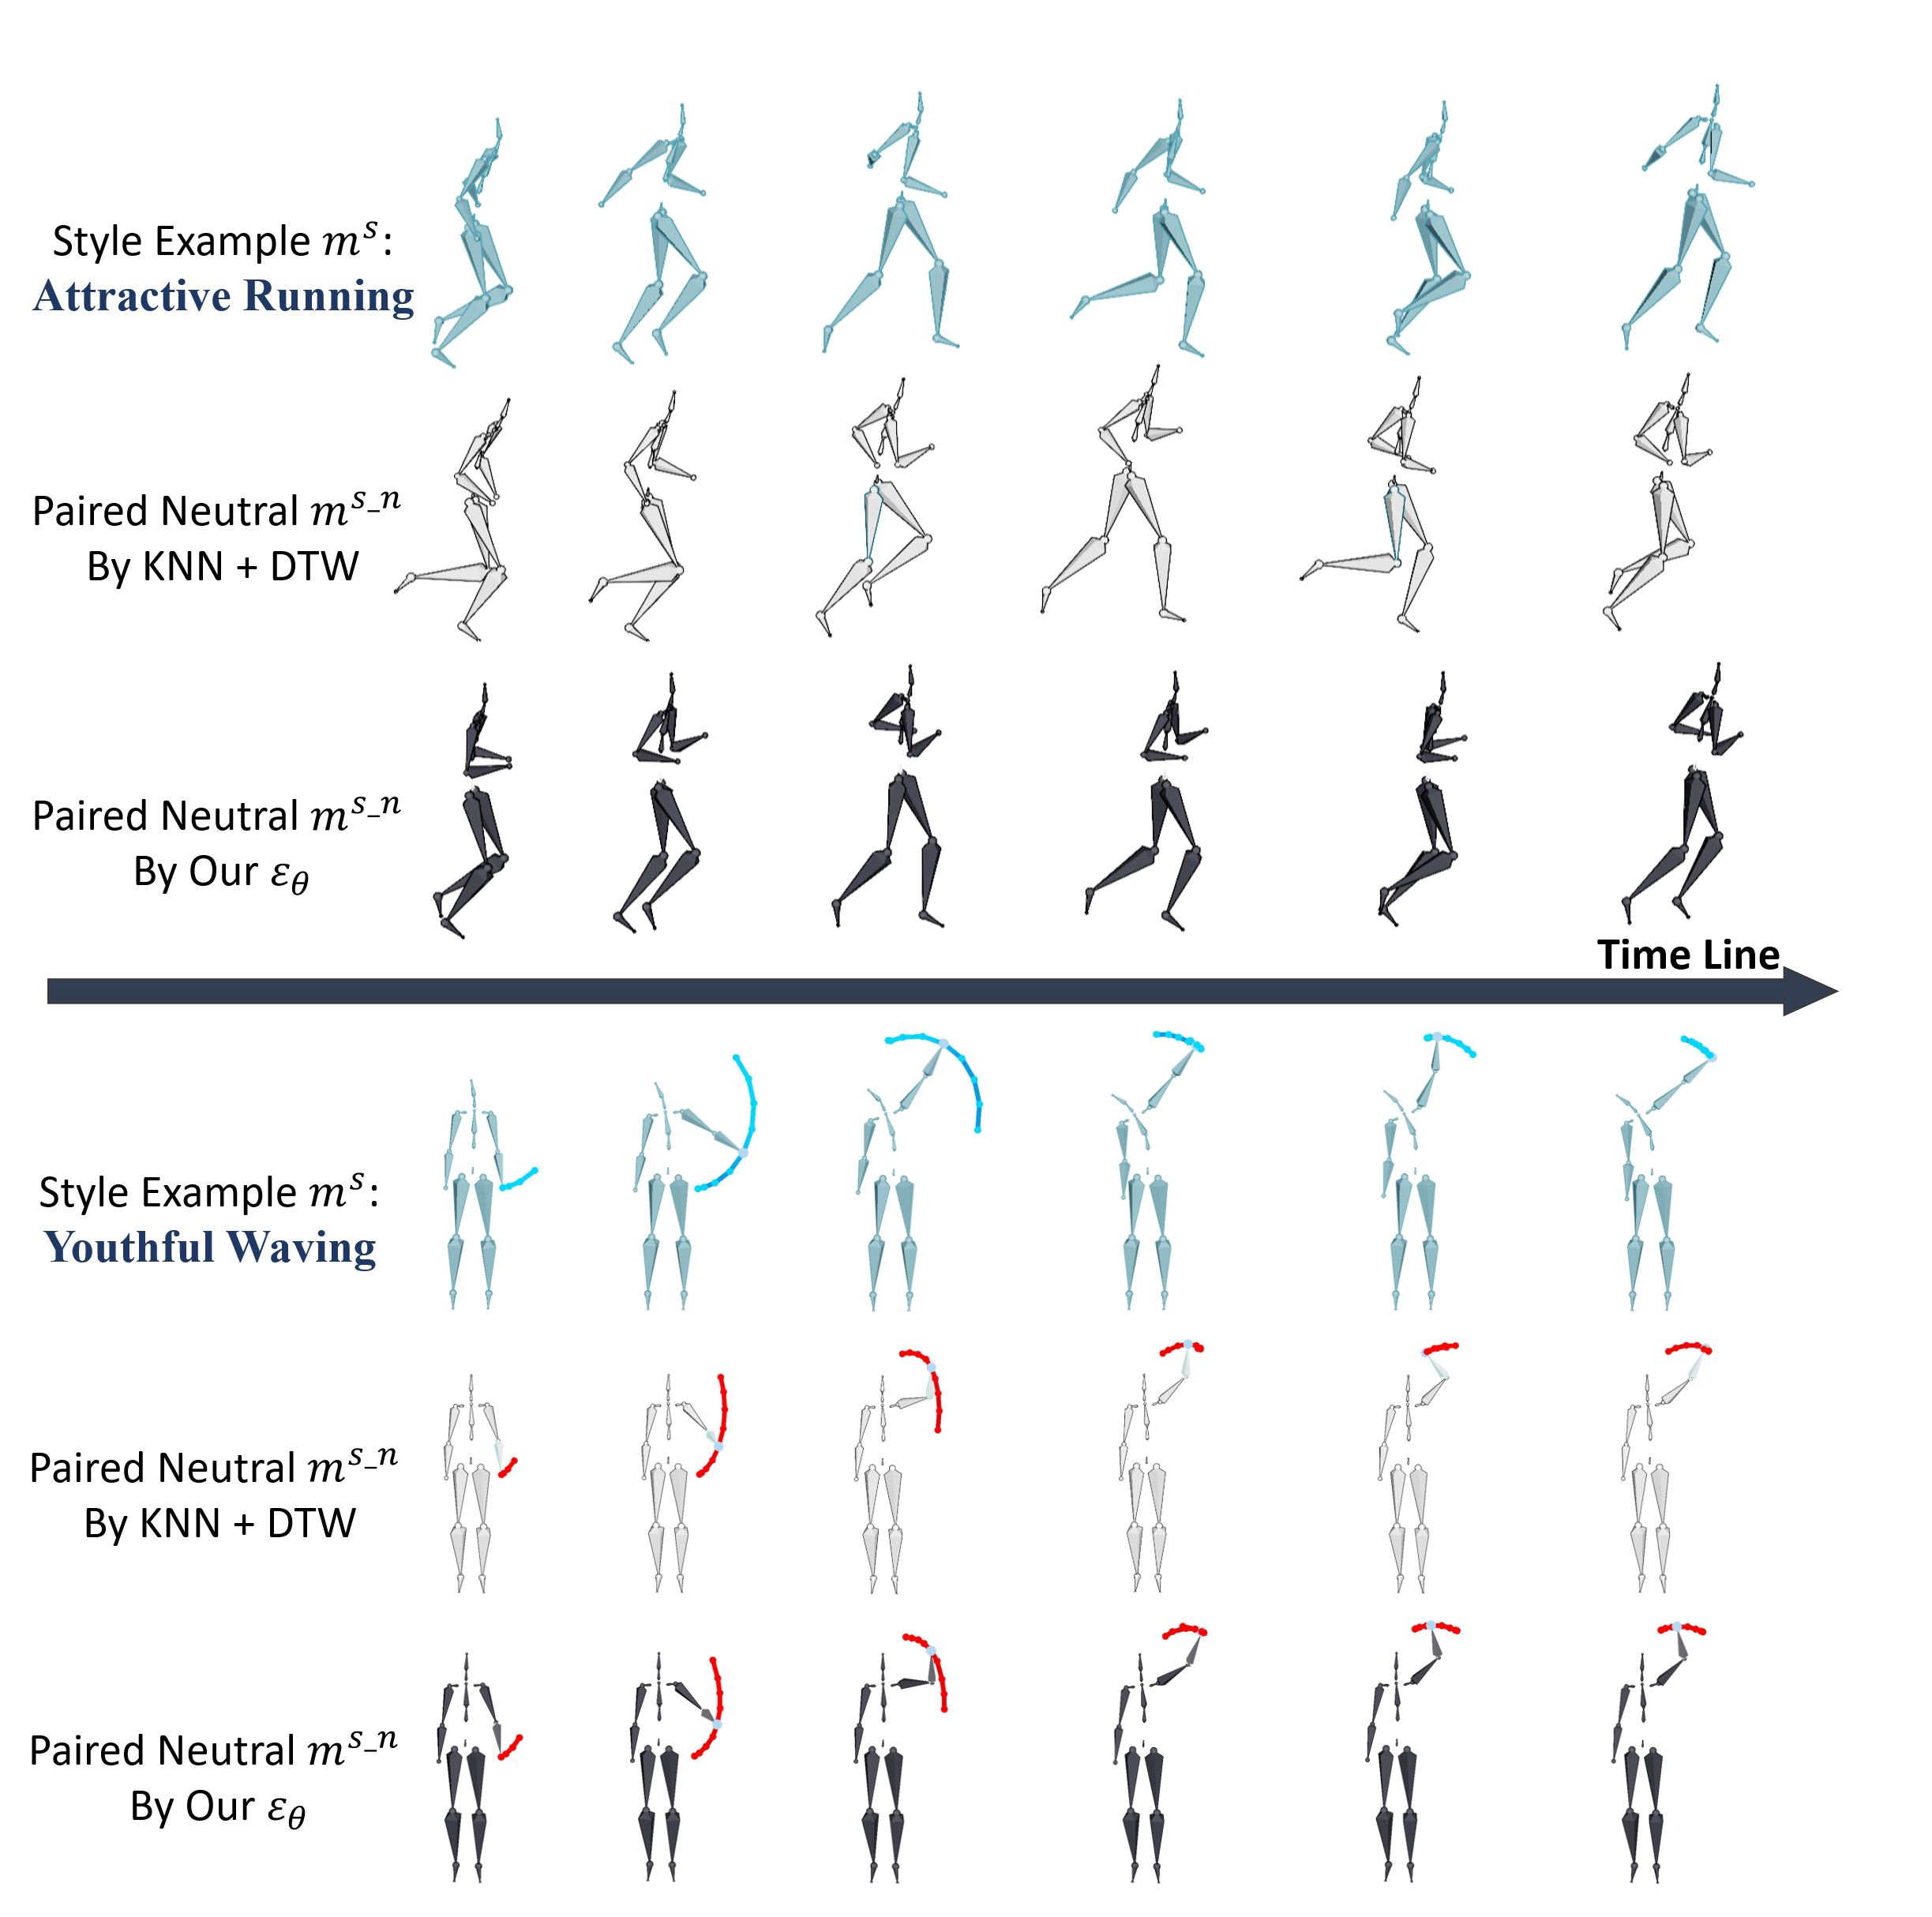}
    \caption{Qualitative evaluation on style-neutral motion pair generation. We compare our method with KNN+DTW. The curve in the figure represents the trajectory of the end-effector between -0.2s$\sim$0.2s.}
    \label{fig:style_neutral_pairs}
\end{figure}

\begin{figure*}[ht]
    \centering
    \includegraphics[width=1\linewidth]{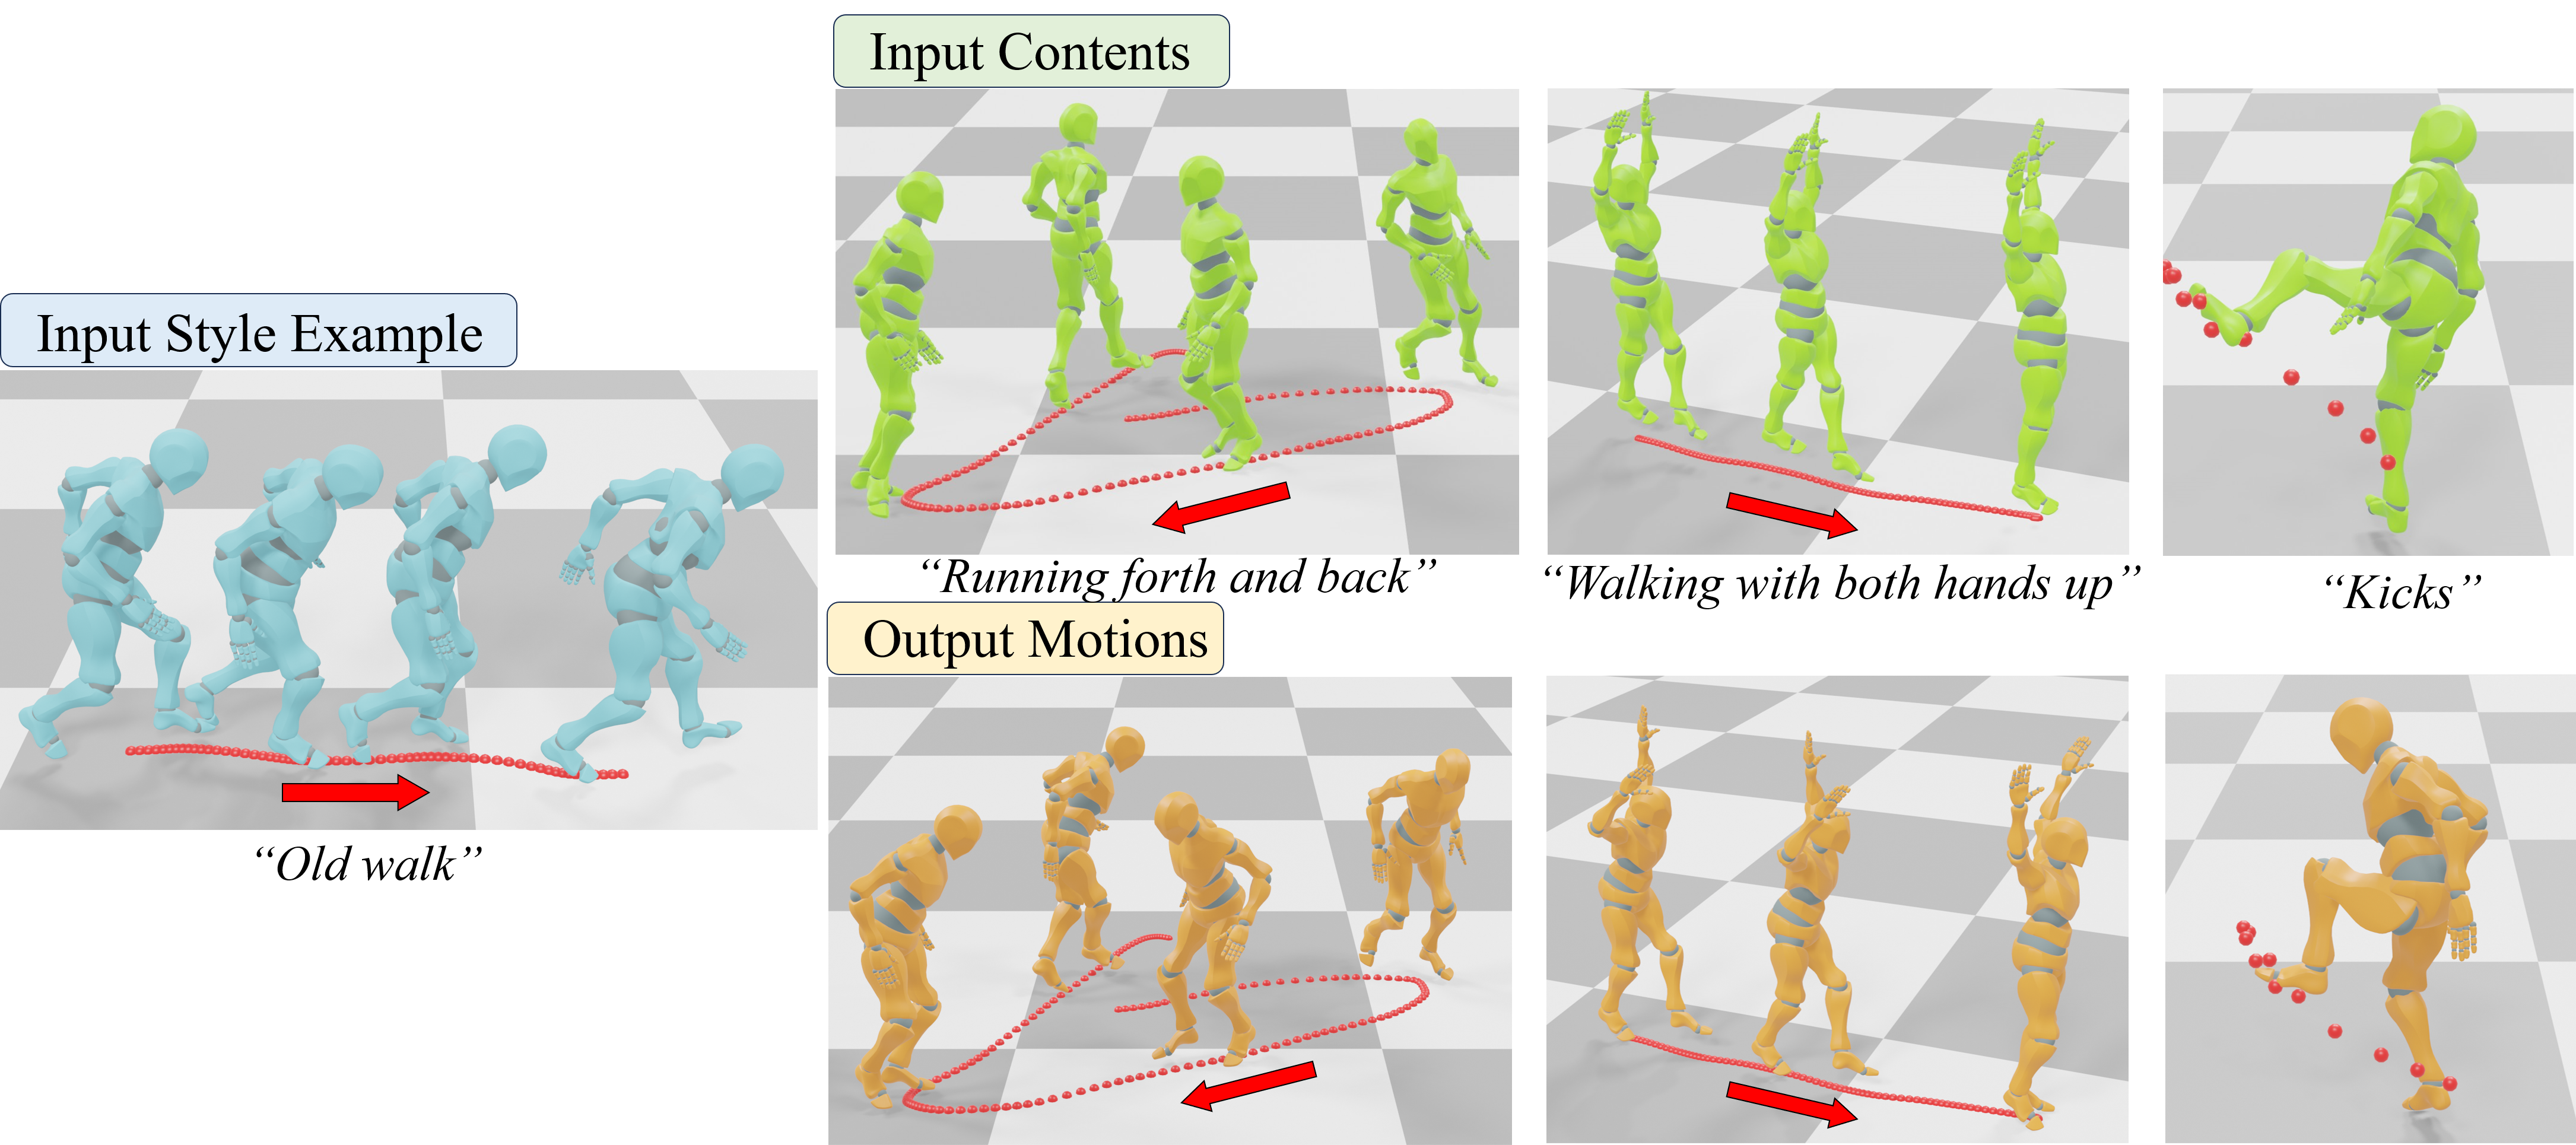}
    \caption{Transfer the "old" style provided by the example to heterogeneous motions}
    \label{fig:teaser}
\end{figure*}

\section{Time Efficiency of Our System}
\label{sec:fine_tune_efficiency}
We test the time efficiency of our framework. The mean pre-training and fine-tuning time of each model on different training datasets is shown in Table~\ref{tab:efficiency}. The time depends on the dataset's scale, and the time of pre-training the motion-semantic discriminator $Dis$ is also relevant to the complexity of the text descriptions. It can be observed that the fine-tuning of $\varepsilon_{\theta s}$ is very efficient, and only takes about 3 minutes even on the HumanML3D trainset. We only fine-tune the model $\varepsilon_{\theta s}$ for one epoch. In this epoch, the training data from the dataset is randomly fed into the network in batch form, while $\mathcal{L}_{sr}$ and $\mathcal{L}_s$ simultaneously supervise the learning. 

\begin{table}[t]
    \centering
    \begin{tabular}{c|c|c|c}     & pre-train $\varepsilon_{\theta}$ & pre-train $Dis$  & fine-tune
    $\varepsilon_{\theta}\rightarrow \varepsilon_{\theta s}$\\
        \hline
        Xia  & 5h 41m & 10m 3s & 17s  \\
        Bandai-2 & 8h 5m & 15m 50s & 1m 5s \\
        HumanML3d & 25h 51m & 29h 46m&3m 10s  \\
        \hline    
    \end{tabular}
    \caption{The time efficiency of our style transfer system on different training datasets. All experiments were tested on a single 3090Ti.}
    \label{tab:efficiency}
\end{table}

\section{Transfer Unseen Style to Heterogeneous Motions}
As Figure~\ref{fig:teaser} shown, we can transfer the unseen style "old" (from Xia Test Set) to heterogeneous content motions. It is worth noting that these content motions are generated from scratch by the T2M generative model $\varepsilon_\theta$ as well as textual guidance, and the model $\varepsilon_\theta$ is only pre-trained on the training set of HumanML3D.
